# Supplementary material for: Signatures of van der Waals binding: a coupling-constant scaling analysis
Source: arXiv:1710.00527 source file (2018-02-20)
Supplement: Supplementary file 1 [file SI.pdf]

# Supplementary materials –
# Signatures of van der Waals binding: a coupling-constant scaling analysis

Yang Jiao, Elsebeth Schröder, and Per Hyldgaard
*Department of Microtechnology and Nanoscience (MC2), Chalmers University of Technology, SE-41296 Gothenburg, Sweden*

TABLE S.I. Binding energy contributions arising from the Kohn-Sham kinetic-energy ($\Delta T_{\rm KS}$), the kinetic-correlation energy ($\Delta T_{\rm c}$), the non-local correlation energy ($\Delta E_{\rm c}^{\rm nl}$), and the non-local kinetic-correlation energy ($\Delta T_{\rm c}^{\rm nl}$) as obtained by our coupling-constant analysis for the vdW-DF-cx functional. The table lists our results in eV for the 19 molecules, for which there also exists a corresponding PBE-based coupling-constant analysis.[1] $\Delta T_{\rm KS}$ is calculated as Kohn-Sham kinetic-energy difference between the isolated atoms and the molecule, $\Delta T_{\rm KS} = \sum_i T_{\rm KS,atom_i} - T_{\rm KS,molecule}$. $\Delta T_{\rm c}$, $\Delta E_{\rm c}^{\rm nl}$ and $\Delta T_{\rm c}^{\rm nl}$ are defined in the same way.

| | $\Delta T_{\rm KS}$ | $\Delta T_{\rm c}$ | $\Delta E_{\rm c}^{\rm nl}$ | $\Delta T_{\rm c}^{\rm nl}$ |
|---|---|---|---|---|
| $H_2$ | -4.3 | -0.69 | -0.210 | 0.108 |
| LiH | -1.9 | -0.55 | -0.192 | 0.092 |
| $CH_4$ | -34.6 | -2.39 | -0.318 | 0.083 |
| $NH_3$ | -26.5 | -2.17 | -0.353 | 0.113 |
| OH | -8.7 | -0.77 | -0.153 | 0.058 |
| $H_2O$ | -20.3 | -1.44 | -0.207 | 0.060 |
| HF | -11.9 | -0.72 | -0.085 | 0.020 |
| $Li_2$ | 0.1 | -0.29 | -0.128 | 0.038 |
| LiF | -14.0 | -0.72 | -0.093 | 0.028 |
| HCN | -27.9 | -1.91 | -0.214 | 0.032 |
| $N_2$ | -11.7 | -1.63 | -0.251 | 0.067 |
| $O_2$ | -8.8 | -0.95 | 0.054 | -0.099 |
| $F_2$ | -0.9 | -0.58 | 0.102 | -0.109 |
| $Cl_2$ | -3.5 | -0.53 | 0.244 | -0.193 |
| $C_2H_2$ | -43.3 | -2.17 | -0.164 | -0.014 |
| $C_2H_4$ | -54.0 | -3.19 | -0.216 | -0.031 |
| CO | -17.8 | -1.16 | -0.058 | -0.029 |
| NO | -15.9 | -1.35 | -0.102 | -0.015 |
| $P_2$ | -1.3 | -1.26 | -0.122 | -0.033 |

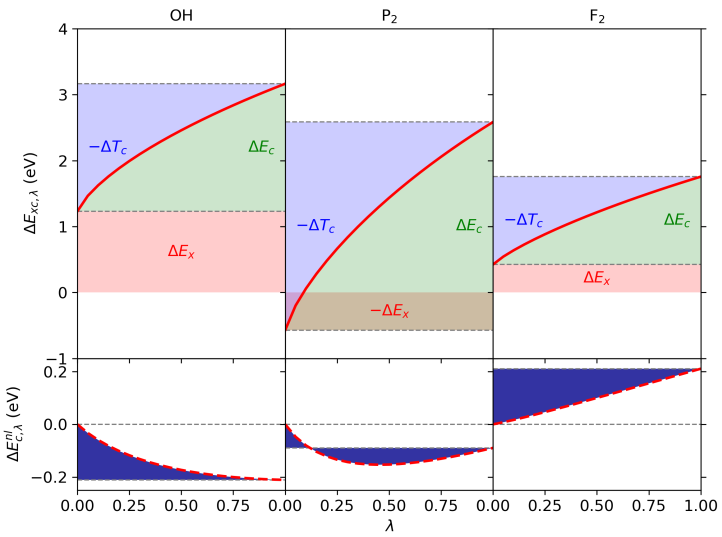


FIG. S.1. Coupling constant scaling of exchange correlation and nonlocal correlation contribution to atomization energies. Example molecules are taken from each of the subgroups in Table S.I. Note that the binding contribution from exchange is negative in the case of $P_2$, and therefore drawn as a shaded area.

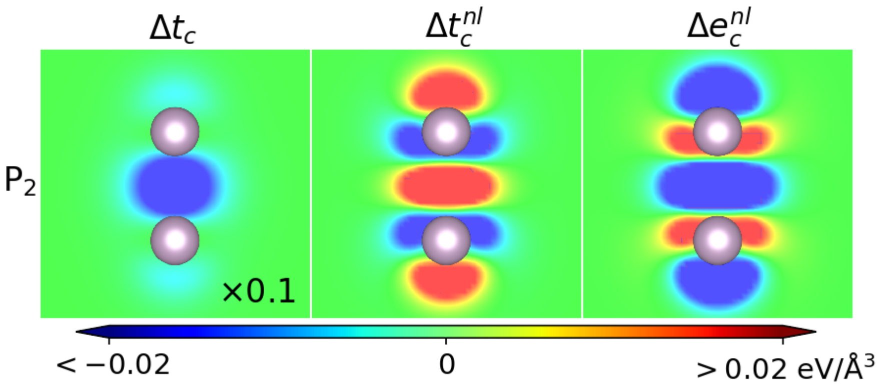


FIG. S.2. Kinetic-energy contributions to the atomization energy for $P_2$ molecule. The color map is the energy density in eV/Å$^3$ as in Figure 4. $\Delta t_c^{nl}$ and $\Delta e_c^{nl}$ are roughly a negative print of each other but with space dependent scale.

TABLE S.II. Binding energy contributions arising from the Kohn-Sham kinetic energy ($\Delta T_{\rm KS}$), the kinetic-correlation energy ($\Delta T_{\rm c}$), the non-local correlation energy ($\Delta E_{\rm c}^{\rm nl}$), and the non-local kinetic-correlation energy ($\Delta T_{\rm c}^{\rm nl}$) as obtained by our coupling-constant analysis of vdW-DF-cx. The table lists our results in eV for molecules in the G2-1 set, omitting the cases that have already been characterized in Table S.I.

| | $\Delta T_{\rm KS}$ | $\Delta T_{\rm c}$ | $\Delta E_{\rm c}^{\rm nl}$ | $\Delta T_{\rm c}^{\rm nl}$ |
|---|---|---|---|---|
| BeH | -8.5 | -0.32 | -0.028 | 0.022 |
| $CH_{2s_3B_1d}$ | -22.9 | -1.02 | -0.097 | 0.014 |
| $CH_{2s_1A_1d}$ | -21.6 | -0.98 | -0.085 | 0.005 |
| $CH_3$ | -28.9 | -1.74 | -0.231 | 0.063 |
| NH | -7.0 | -0.76 | -0.153 | 0.060 |
| $NH_2$ | -15.7 | -1.48 | -0.274 | 0.099 |
| $SiH_{2s_1A_1d}$ | -6.4 | -1.12 | -0.243 | 0.096 |
| $SiH_{2s_3B_1d}$ | -7.6 | -0.86 | -0.112 | 0.033 |
| $SiH_3$ | -10.8 | -1.48 | -0.249 | 0.088 |
| $SiH_4$ | -14.0 | -2.06 | -0.372 | 0.139 |
| $PH_2$ | -6.6 | -1.26 | -0.235 | 0.072 |
| $PH_3$ | -10.1 | -1.85 | -0.326 | 0.097 |
| $SH_2$ | -7.3 | -1.19 | -0.151 | 0.027 |
| $N_2H_4$ | -46.7 | -3.73 | -0.338 | 0.012 |
| $Na_2$ | 0.5 | -0.25 | -0.094 | 0.020 |
| $Si_2H_6$ | -23.6 | -3.52 | -0.406 | 0.082 |
| CH | -16.8 | -0.19 | 0.073 | -0.056 |
| $CO_2$ | -41.8 | -2.06 | 0.035 | -0.135 |
| $Si_2$ | -2.7 | -0.59 | 0.037 | -0.069 |
| $S_2$ | -4.8 | -0.73 | 0.179 | -0.167 |
| NaCl | -3.6 | -0.54 | 0.007 | -0.034 |
| CS | -7.3 | -0.96 | 0.016 | -0.077 |
| SO | -11.1 | -0.87 | 0.095 | -0.114 |
| ClO | -6.5 | -0.77 | 0.115 | -0.125 |
| ClF | -6.9 | -0.58 | 0.161 | -0.143 |
| HOCl | -14.6 | -1.34 | 0.069 | -0.124 |
| $SO_2$ | -27.3 | -1.90 | 0.154 | -0.212 |
| HCl | -4.0 | -0.58 | -0.044 | -0.004 |
| $C_2H_6$ | -64.5 | -4.21 | -0.260 | -0.052 |
| CN | -23.8 | -1.31 | -0.106 | -0.006 |
| HCO | -28.6 | -1.59 | -0.055 | -0.053 |
| $H_2CO$ | -36.4 | -2.19 | -0.134 | -0.029 |
| $CH_3OH$ | -49.4 | -3.22 | -0.177 | -0.056 |
| $H_2O_2$ | -24.0 | -2.14 | -0.094 | -0.062 |
| SiO | -11.4 | -1.04 | -0.073 | -0.013 |
| $CH_3Cl$ | -33.3 | -2.37 | -0.008 | -0.123 |
| $CH_3SH$ | -37.2 | -3.00 | -0.105 | -0.099 |

TABLE S.III. Non-covalent binding energy contributions for dimers from the S22 dataset as obtained from our coupling-constant scaling of the vdW-DF-cx functional (Energy unit: eV). The table lists contributions arising from the Kohn-Sham kinetic-energy ($\Delta T_{\mathrm{KS}}$), the kinetic-correlation energy ($\Delta T_{\mathrm{c}}$), the non-local correlation energy ($\Delta E_{\mathrm{c}}^{\mathrm{nl}}$), and the non-local kinetic-correlation energy ($\Delta T_{\mathrm{c}}^{\mathrm{nl}}$), $\Delta T_{KS}$ is calculated as the Kohn-Sham kinetic-energy difference between isolated molecules and the dimer, $\Delta T_{\mathrm{KS}} = \sum_i T_{\mathrm{KS,molecule_i}} - T_{\mathrm{KS,dimer}}$. $\Delta T_{\mathrm{c}}$, $\Delta E_{\mathrm{c}}^{\mathrm{nl}}$ and $\Delta T_{\mathrm{c}}^{\mathrm{nl}}$ are defined in the same way. The characterization is separated into three parts: complexes that are hydrogen bonded, dispersion bonded, or with a mixed binding.

| | $\Delta T_{\mathrm{KS}}$ | $\Delta T_{\mathrm{c}}$ | $\Delta E_{\mathrm{c}}^{\mathrm{nl}}$ | $\Delta T_{\mathrm{c}}^{\mathrm{nl}}$ |
|---|---|---|---|---|
| Ammonia dimer | -0.582 | -0.080 | 0.077 | -0.056 |
| Water dimer | -1.322 | -0.087 | 0.070 | -0.053 |
| Formic acid dimer | -6.253 | -0.299 | 0.232 | -0.168 |
| Formamide dimer | -4.199 | -0.256 | 0.215 | -0.153 |
| Uracil dimer h-bonded | -4.134 | -0.290 | 0.269 | -0.188 |
| 2-pyridoxine 2-aminopyridine complex | -3.722 | -0.299 | 0.284 | -0.197 |
| Adenine-thymine Watson-Crick complex | -3.708 | -0.321 | 0.315 | -0.216 |
| Methane dimer | -0.100 | -0.049 | 0.060 | -0.041 |
| Ethene dimer | -0.323 | -0.110 | 0.127 | -0.088 |
| Benzene-methane complex | -0.186 | -0.117 | 0.144 | -0.098 |
| Benzene dimer parallel displaced | -0.298 | -0.303 | 0.396 | -0.263 |
| Pyrazine dimer | -0.631 | -0.327 | 0.417 | -0.280 |
| Uracil dimer stack | -1.038 | -0.470 | 0.601 | -0.403 |
| Indole-benzene complex stack | -0.242 | -0.432 | 0.568 | -0.377 |
| Adenine-thymine complex stack | -0.958 | -0.657 | 0.847 | -0.568 |
| Ethene-ethyne complex | -0.140 | -0.058 | 0.065 | -0.044 |
| Benzene-water complex | -0.547 | -0.125 | 0.140 | -0.098 |
| Benzene-ammonia complex | -0.332 | -0.120 | 0.142 | -0.097 |
| Benzene-HCN complex | -0.554 | -0.153 | 0.173 | -0.119 |
| Benzene dimer T-shaped | -0.285 | -0.182 | 0.230 | -0.154 |
| Indole-benzene T-shape complex | -0.592 | -0.253 | 0.312 | -0.209 |
| Phenol dimer | -1.740 | -0.247 | 0.283 | -0.193 |

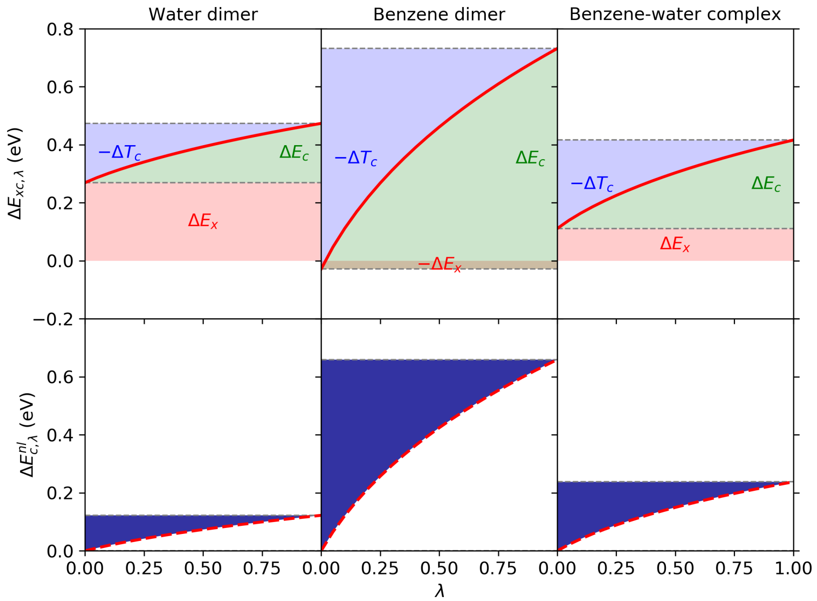


FIG. S.3. Coupling constant scaling of exchange correlation and non-local correlation contribution to binding energies.

[1] K. Burke, M. Ernzerhof, and J. P. Perdew, Chem. Phys. Lett. **265**, 115 (1997).

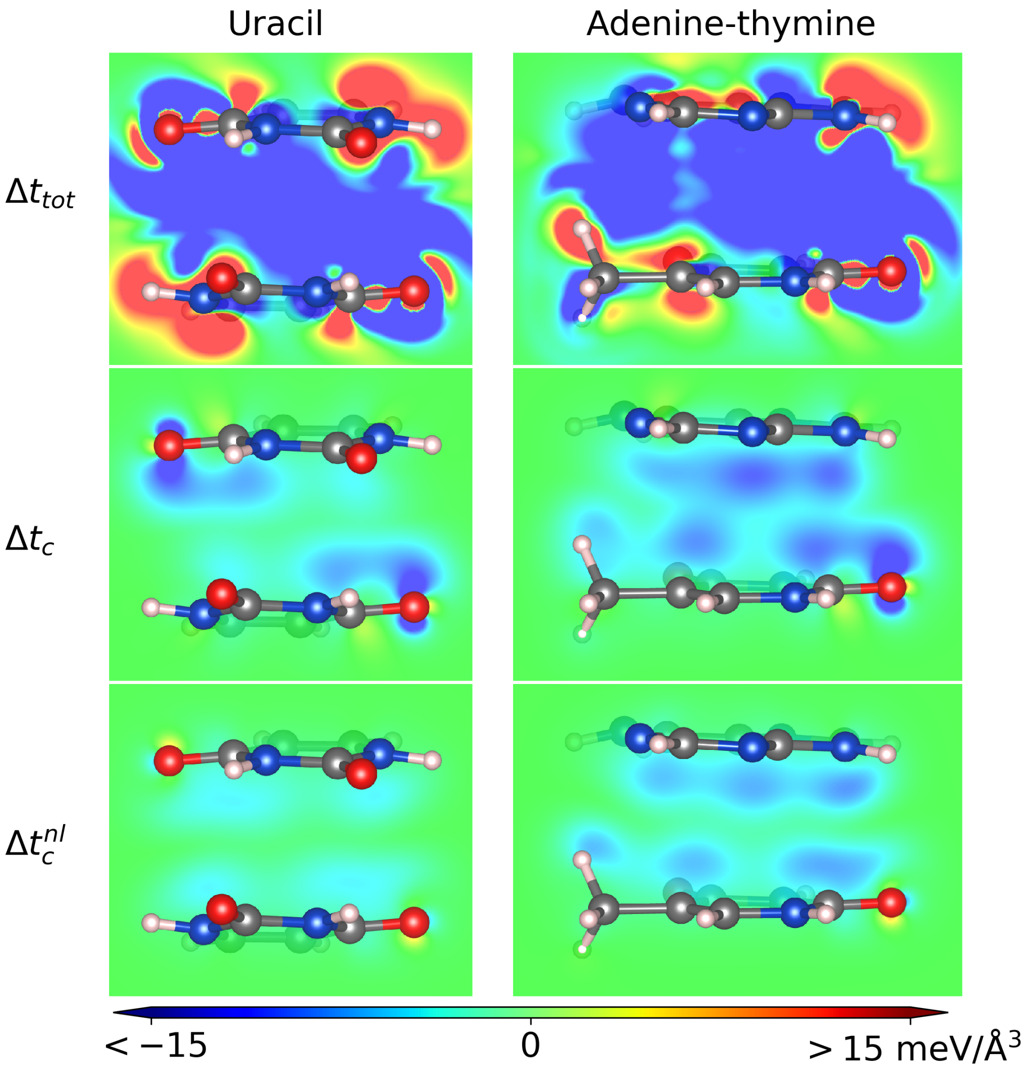


FIG. S.4. Spatial variation in binding contributions to the stacked uracil dimer (left column of panels) and to the stacking of adenine and thymine bases (right column of panels). All configurations are the same as in Figure 6. The panels in the first (second) row show the binding contributions in the total kinetic (in the kinetic-correlation) energy. The panels in the third row show the binding contribution $\Delta t_c^{\rm nl}$ from the nonlocal part of the kinetic-correlation energy in vdW-DF-cx functional description.
